# Supplementary material for: DocuMint: Docstring Generation for Python using Small Language Models
Source: arXiv:2405.10243 source file (2024-05-16)
Supplement: Supplementary file 2 [file appendix.tex]

\begin{figure}[h!]
    \centering
    \includegraphics[]{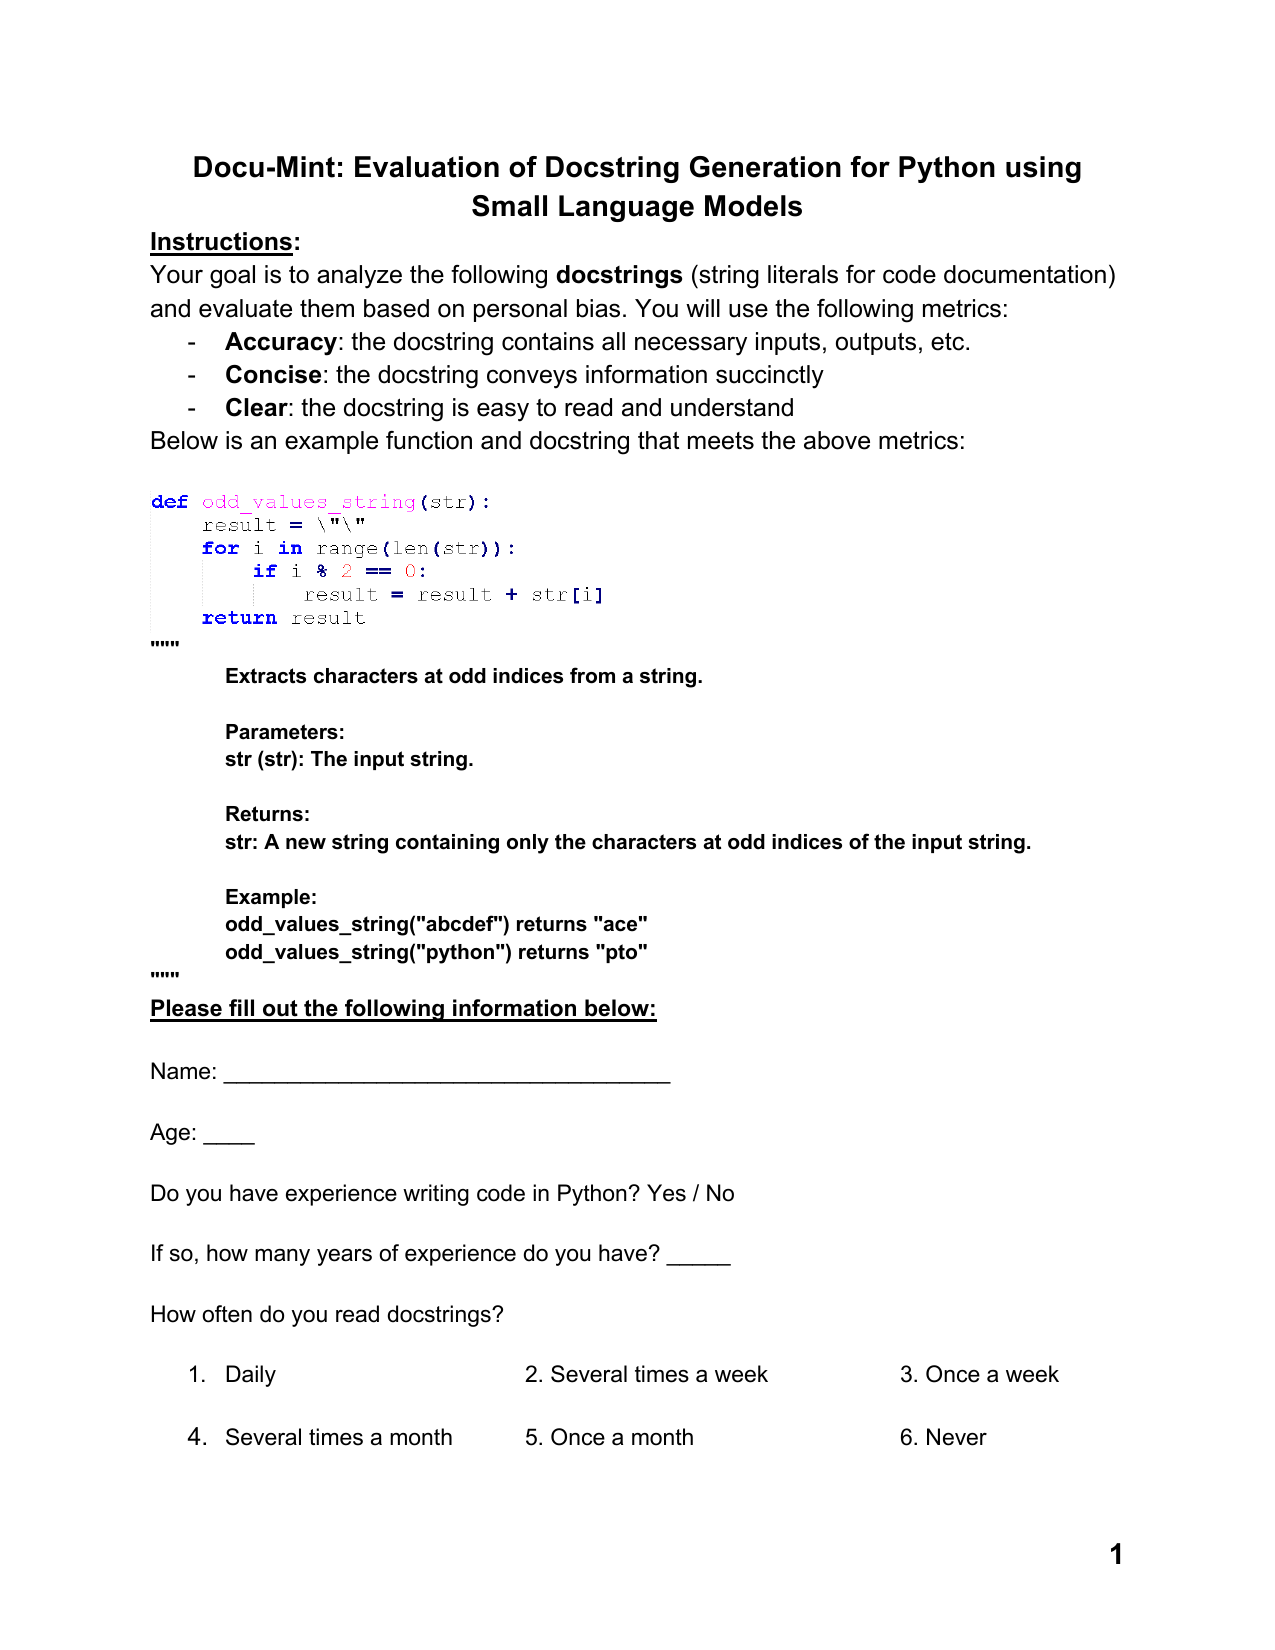}\\
    \caption{}
    \label{sample_questionnaire}
\end{figure}
